# Supplementary material for: Classification with Partially Private Features
Source: arXiv:2312.07583 source file (2023-12-11)
Supplement: Supplementary file 1 [file appendix.tex]

\centerline {\LARGE \bf Supplementary Material}
